# Supplementary material for: Lipschitz constant estimation of Neural Networks via sparse polynomial optimization
Source: arXiv:2004.08688 source file (2020-04-18)
Supplement: Supplementary file 1 [file appendix1.tex]

\begin{lemma}
Let $p(x) = a_0 + \sum_{i=1}^d a_i x_i + \sum_{i \leq j} a_{ij}x_i x_j$ be a polynomial of degree $2$. Suppose that there exists a decomposition 
\begin{equation}
p(x) = \sum_{(\alpha, \beta) \in \N_{k}^{2m}} c_{\alpha\beta}\prod_{j=1}^m x_j^{\alpha_j}(1-x_j)^{\beta_j},
\label{eq:poly-decomp}
\end{equation}
where $c_{\alpha \beta} \geq 0$, and $k=2$. Then, we can find a similar decomposition that satisfies $\forall i \geq j$:
\begin{equation*}
a_{ij} = 0 \Rightarrow c_{\{i,j\} \emptyset} = c_{\emptyset \{i,j\} } = c_{\{i\} \{j\}} = c_{\{j\} \{i\}} = 0
\end{equation*}
\end{lemma}

\begin{proof}
Suppose that $\exists i \leq j$ such that $a_{ij} = 0$. This means that the term in the decomposition~\eqref{eq:poly-decomp} corresponding to the factor $x_i x_j$ has coefficient $0$. 

In order to prove the theorem, we need to show that there exists a polynomial of the form~\eqref{eq:poly-decomp} where $c_{\{i,j\} \emptyset} = c_{\emptyset \{i,j\} } = c_{\{i\} \{j\}} = c_{\{j\} \{i\}} = 0$. To do so, we show that under the condition $a_{ij} = 0$, the contributions from these four terms in~\eqref{eq:poly-decomp} can be rewritten as lower order  terms with positive coefficients, i.e., $\exists a,b,c,d,e \geq 0$ such that
\begin{equation}
\begin{split}
 &c_{\{i,j\} \emptyset}x_ix_j + c_{\{i\} \{j\}}x_i(1-x_j) + c_{\{j\} \{i\}}x_j(1-x_i) + c_{\emptyset \{i,j\} }(1-x_i)(1-x_j) \\
 &= a x_i + b (1-x_i) + c x_j + d (1-x_j) + e.
\end{split}
\label{eq:term-decomp}
\end{equation}

If we track the contributions to the $x_i x_j$ term in the decomposition, the condition $a_{ij} = 0$ is equivalent to:
\begin{equation}
 c_{\{i,j\} \emptyset} - c_{\{i\} \{j\}} - c_{\{j\} \{i\}} + c_{\emptyset \{i,j\} } = 0
 \label{eq:sparsity}
\end{equation}

Under~\eqref{eq:sparsity} condition, the left end side of~\eqref{eq:term-decomp} can be written as:
\begin{align*}
&c_{\{i,j\} \emptyset}x_ix_j - c_{\{i\} \{j\}}x_i(1-x_j) - c_{\{j\} \{i\}}x_j(1-x_i) + c_{\emptyset \{i,j\} }(1-x_i)(1-x_j) \\
&= c_{\{i\} \{j\}}x_i + c_{\{j\} \{i\}}x_j + c_{\emptyset \{i,j\} }(1-x_i-x_j)
\end{align*}

In order to rewrite this last equation in the form of the right hand side of~\eqref{eq:term-decomp}, note that:
\begin{align}
&c_{\{i\} \{j\}}x_i + c_{\{j\} \{i\}}x_j + c_{\emptyset \{i,j\} }(1-x_i-x_j) = \nonumber \\
&\begin{cases}
(c_{\{i\} \{j\}} - c_{\emptyset \{i,j\} }) x_1 + (c_{\{j\} \{i\}} - c_{\emptyset \{i,j\} })x_2 + c_{\emptyset \{i,j\} }, \text{ if } c_{\emptyset \{i,j\} } \leq c_{\{i\} \{j\}}, c_{\{j\} \{i\}} \\
(c_{\emptyset \{i,j\} } - c_{\{i\} \{j\}}) (1 - x_1) + (c_{\emptyset \{i,j\} } - c_{\{j\} \{i\}})(1 - x_2) + c_{\{i\} \{j\}} + c_{\{j\} \{i\}} -c_{\emptyset \{i,j\} }, \text{ if } c_{\emptyset \{i,j\} } \geq c_{\{i\} \{j\}}, c_{\{j\} \{i\}} \\
(c_{\{i\} \{j\}} - c_{\emptyset \{i,j\} }) x_1 + (c_{\emptyset \{i,j\} } - c_{\{j\} \{i\}})(1 - x_2) + c_{\{j\} \{i\}}, \text{ if } c_{\{j\} \{i\}} \leq c_{\emptyset \{i,j\} } \leq c_{\{i\} \{j\}} \\
(c_{\emptyset \{i,j\} } - c_{\{i\} \{j\}}) (1 - x_1) + (c_{\{j\} \{i\}} - c_{\emptyset \{i,j\} })x_2 + c_{\{i\} \{j\}}, \text{ if } c_{\{i\} \{j\}} \leq c_{\emptyset \{i,j\} } \leq c_{\{j\} \{i\}}
\end{cases}
\label{eq:linear-decomp}
\end{align}

Finally, note that the condition~\eqref{eq:sparsity} together with the fact that $c_{\{i,j\} \emptyset} \geq 0$ implies that $c_{\{i\} \{j\}} + c_{\{j\} \{i\}} - c_{\emptyset \{i,j\} } \geq 0$ so that the constant term in the second line of~\eqref{eq:linear-decomp} is also non-negative.

\end{proof}
