# Supplementary material for: Lipschitz constant estimation of Neural Networks via sparse polynomial optimization
Source: arXiv:2004.08688 source file (2020-04-18)
Supplement: Supplementary file 2 [file appendix_qcqp.tex]

explain the matrix $H(W_1,W_2,v)$
